# Supplementary material for: A New Broadcast Primitive for BFT Protocols
Source: arXiv:2410.22080 source file (2024-10-30)
Supplement: Supplementary file 1 [file appendix.tex]

\appendix
\section{RTT Measurements}
\label{appendix:rtts}

\begin{table*}
    \footnotesize
    \begin{tabular}{|c|cccccccccccc|}
        \hline
        \input{rtt-table}\\
        \hline
    \end{tabular}
    \caption{RTT measurements between a subset of datacenter contributing to the IC mainnet network (in milliseconds). All nodes are connected over the public IPv6 Internet, without any dedicated links.
    \label{tbl:rtt}}
\end{table*}
